# Supplementary material for: Effective Field Theory Approach to General Relativity and Feynman Diagrams for Coalescing Binary Systems
Source: arXiv:2211.01321 source file (2022-10-16)
Supplement: Supplementary file 1 [file Appendix_B.tex]

\chapter{Alternative derivation of the Low-Energy limit}
\label{appendix:Alternative_derrivation}
In this section we present the results obtained and we compare them with the ones obtained in \cite{Bjerrum-Bohr:2014zsa}\cite{Bjerrum-Bohr:2016hpa}. 
In the previous section we explained how to get the expression for the 1-loop amplitude using Feynman diagrams, obtaining an expression for the total amplitude in terms of four Master Integrals:
\begin{equation}
    \kappa^{-4}\mathcal{M}^{1-loop}(p_1,p_2,p_3,p_4)= AI_{\Box}+BI_{\times}+CI_{\lhd}+DI_{\bigcirc}
\end{equation}
Working in $d$ dimensions we found the following expressions for the coefficients:
\begin{equation}
\begin{split}
   & A= \frac{1}{16}(m^2-t)^4\\
   & B= \frac{1}{16}(m^2-u)^4 \\
   & C=\frac{1}{16(2m^2+t+u)^2)}\biggl(6m^6(t-u)-6m^8(t+u)-3m^2(t^2-u^2)^2-(t+u)^3(t^2-tu+u^2)\\
   & +m^4(t^3+9t^2u+9tu^2+u^3)\biggr) \\
   & D = \frac{1}{16\epsilon}(m^4-m^2t+t^2-m^2u-tu+u^2)+\frac{1}{1920(2m^2+t+u)^2}\bigl(3664m^8+864m^6t-1712m^4t^2-92t^4\\ &+864m^6u
   -1936m^4tu +24m^2t^2u+424t^3u-1712m^4u^2+24m^2tu^2+1032t^2u^2-888m^2u^3+24tu^3-92u^4) \\
\end{split}
\end{equation}
They match exactly with the ones obtained in \cite{Bjerrum-Bohr:2016hpa}\cite{Bjerrum-Bohr:2014zsa} once we decompose the massless triangle integral present in their result in terms of our basis of Master Integrals. \\
\section{Low-energy limit}
We can study the low-energy non-relativistic limit of this amplitude, where the energy $E$ of the massless particle is much smaller than the mass of the massive scalar $E\ll M$ and the momentum transfer $s\approx -\mathbf{q}^2$ is tiny as well. \\ 
We have to apply the following approximations to our amplitude:
\begin{equation}
    s=(p_1+p_2)^2 \approx -\mathbf{q^2} \quad t=(p_1+p_3)^2\approx m^2+2E m \quad u=(p_1+p_4)^2 \approx m^2-2E m+\mathbf{q}^2
\end{equation}
Moreover we will be interested in the small angle scattering approximation: $s \ll E^2$. \\
In order to do that first of all we take the asymptotic limit of each coefficient multiplying the Master Integrals obtaining:
\begin{equation}
     \kappa^{-4}\mathcal{M}^{1-loop}(p_1,p_2,p_3,p_4)= E^2m^2\biggl((Em)^2(I_{\Box}+I_{\times})-\frac{15}{16}I_{\lhd}+\biggl(-\frac{237}{160}+\frac{3}{4\epsilon}\biggr)I_{\bigcirc}
\end{equation}
Then we substitute the expressions for the Master Integrals in the non-relativistic limit which are:
\begin{equation}
\begin{split}
    & I_{\bigcirc}\approx -\frac{1}{16\pi^2}\biggl(2-log\biggl(\frac{-s}{\mu^2}\biggr)\biggr)\qquad I_{\lhd}\approx-\frac{1}{32\pi^2m^2}\biggl(log\biggl(\frac{-s}{m^2}\biggr)+\frac{\pi^2m}{\sqrt{-s}}\biggr) \qquad I_{\Box}+I_{\times}\approx \frac{i}{8\pi s m E}log\biggl(\frac{-s}{m^2}\biggr)\\
\end{split}    
\end{equation}
obtaining:
\begin{equation}
    \kappa^{-4}\mathcal{M}^{1-loop}=(m E)^2\biggl[+\frac{15}{512}\frac{m}{\sqrt{-q^2}}+\frac{15}{512\pi^2}log\biggl(\frac{-q^2}{m^2}\biggr)-\frac{3}{2560\pi^2}log\biggl(\frac{-q^2}{\mu^2}\biggr)-\frac{3}{128\pi^2}log^2\biggl(\frac{-q^2}{\mu^2}\biggr)+\frac{m E}{8\pi q^2}log\biggl(\frac{-q^2}{m^2}\biggr)\biggr]
\end{equation}
Also this result agree with \cite{Bjerrum-Bohr:2016hpa}.
The total amplitude at 1-loop is, writing $E=\hbar w$:
\begin{equation}
\begin{split}
    \mathcal{M}_{TOT}=\mathcal{M}^{tree}+\mathcal{M}^{1-loop}=& \frac{(M\omega)^2}{\hbar}\biggl[-\frac{\kappa^2}{\mathbf{q}^2}+\kappa^4\frac{15}{512}\frac{m}{    \sqrt{\mathbf{q}^2}}+\kappa^4\frac{15\hbar}{512\pi^2}log\biggl(\frac{\mathbf{q^2}}{m^2}\biggr)-\kappa^4\frac{3\hbar}{2560\pi^2}log\biggl(\frac{\mathbf{q}^2}{\mu^2}\biggr)+ \\
    & -\kappa^4\frac{3\hbar}{128\pi^2}log^2\biggl(\frac{\mathbf{q^2}}{\mu^2}\biggr)-\kappa^4\frac{M\omega}{8\pi}\frac{i}{\mathbf{q^2}}log\biggl(\frac{\mathbf{q^2}}{M^2}\biggr)\biggr]
\end{split}
\end{equation}
The explicit expressions for the Master Integrals used for this work have been obtained using \textit{Pakcage-X} and are given by:

\begin{eqnarray}
     I_{1}&=& \frac{i}{16 \pi ^2\epsilon} +\frac{i}{16 \pi ^2} \left(\log \left(-\frac{\bar{\mu}^2}{s}\right)+2\right)-\frac{i \epsilon}{192 \pi ^2}  \left(-6 \log
   ^2\left(-\frac{\bar{\mu}^2}{s}\right)-24 \log \left(-\frac{\bar{\mu}^2}{s}\right)+\pi ^2-48\right)+O\left(\epsilon ^2\right)\\
    I_2&=& \frac{i}{96 \pi ^2 s \sqrt{\frac{s-4
   m^2}{s}}}\left(3 \log ^2\left(\frac{s\left(\sqrt{1-\frac{4 m^2}{s}} -1\right)}{2
   m^2}+1\right)+12 \text{Li}_2\left(\frac{s\left(\sqrt{1-\frac{4 m^2}{s}}-1\right)}{2
   m^2}+1\right)+4 \pi ^2\right)+O\left(\epsilon ^1\right) \\
   I_3&=&\frac{i}{8 \pi ^2 s \left(t-m^2\right)\epsilon ^2}+-\frac{i
   \left(\log \left(-\frac{m^2}{s}\right)+2 \log \left(\frac{\bar{\mu}^2}{m^2-t}\right)\right)}{16 \pi ^2 s \left(m^2-t\right)\epsilon}\nonumber\\
   & &+\frac{i
   \left(2 \pi ^2-3 \left(\log \left(-\frac{m^2}{s}\right)+\log
   \left(\frac{\bar{\mu}^2}{m^2}\right)\right) \left(\log
   \left(\frac{m^2}{m^2-t}\right)+\log \left(\frac{\bar{\mu}^2}{m^2-t}\right)\right)\right)}{48 \pi ^2 s
   \left(m^2-t\right)}+O\left(\epsilon ^1\right) \\
   I_4&=&\frac{i}{8 \pi ^2 s \left(u-m^2\right)\epsilon ^2}+-\frac{i
   \left(\log \left(-\frac{m^2}{s}\right)+2 \log \left(\frac{\bar{\mu}^2}{m^2-u}\right)\right)}{16 \pi ^2 s \left(m^2-u\right)\epsilon}\nonumber\\
   & &+\frac{i
   \left(2 \pi ^2-3 \left(\log \left(-\frac{m^2}{s}\right)+\log
   \left(\frac{\bar{\mu}^2}{m^2}\right)\right) \left(\log
   \left(\frac{m^2}{m^2-u}\right)+\log \left(\frac{\bar{\mu}^2}{m^2-u}\right)\right)\right)}{48 \pi ^2 s
   \left(m^2-u\right)}+O\left(\epsilon ^1\right) 
\end{eqnarray}
where we defined ${\bar{\mu}}^2=4\pi e^{-\gamma_E} \mu^2$, with $\gamma_E$ being the Euler-Mascheroni constant.\\
