# Supplementary material for: Effective Field Theory Approach to General Relativity and Feynman Diagrams for Coalescing Binary Systems
Source: arXiv:2211.01321 source file (2022-10-16)
Supplement: Supplementary file 2 [file Appendix_A.tex]

\chapter{Derivation of the Feynman Rules}
\label{appendix:Feynman_Rules}
We report here the Feynman rules useful to compute 1-loop diagrams, that have been taken from \cite{Holstein:2008sx}\\
In order to find the interaction vertices between scalar fields and gravitons we need to consider the action of a scalar field minimally coupled to gravitons:
\begin{equation}
    S=\int d^4x\sqrt{-g}\biggl(\frac{1}{2}g^{\mu\nu}\partial_{\mu}\phi\partial_{\nu}\phi -\frac{1}{2}m^2\phi^2\biggr)
\end{equation}
and we need to expand it in terms of the gravitational field $h_{\mu\nu}$. \\
This can be done by expanding the metric about flat Minkovski space-time as:
\begin{equation}
    g_{\mu\nu}=\eta_{\mu\nu}+h_{\mu\nu}
\end{equation}
with $\kappa=\sqrt{32\pi G}$.  \\
From the expanded action we can get the Feynman rules describing the interactions of a two-scalar fields with one graviton:\\ 
\begin{equation}
\begin{tikzpicture}[baseline=(current bounding box.center)] \begin{feynman}
\vertex (a) ;
\vertex[below=1.5cm of a] (b);
\vertex[below=1.5cm of b] (c); 
\vertex[right=1.5cm of b] (d){\(\mu\nu\)};
\vertex[below=1cm of d] (e) ;
\vertex[above=1cm of d] (f);
\diagram* { 
(c) -- [fermion, edge label'=\(p_1\)] (b)-- [fermion, edge label'=\(p_2\)] (a),
(b) -- [gluon] (d) ,
};
\end{feynman} \end{tikzpicture}= \tau_{1\mu\nu}(p_1,p_2,m) =  -\frac{i\kappa}{2}\biggl[p_{1\mu}p_{2\nu}+p_{1\nu}p_{2\mu}-\eta_{\mu\nu}(p_1\cdot p_2 -m^2)\biggr]
\end{equation}\\
and with 2 gravitons:
\begin{equation}
\begin{split}
\begin{tikzpicture}[baseline=(current bounding box.center)] \begin{feynman}
\vertex (a) ;
\vertex[below=1.5cm of a] (b);
\vertex[below=1.5cm of b] (c); 
\vertex[right=1.5cm of b] (d);
\vertex[below=1cm of d] (e) {\(\mu\nu\)};
\vertex[above=1cm of d] (f){\(\rho\sigma\)};
\diagram* { 
(c) -- [fermion, edge label'=\(p_1\)] (b)-- [fermion, edge label'=\(p_2\)] (a),
(b) -- [gluon] (e) ,
(b) -- [gluon] (f) ,
};
\end{feynman} \end{tikzpicture}=\tau_{2\mu\nu\rho\sigma}(p_1,p_2)= 
&\frac{i\kappa^2}{2}\biggl[
2I_{\mu\nu\alpha\gamma}I^{\gamma}_{\beta,\rho\sigma}(p_{1}^{\alpha}p_{2}^{\beta}+p_{1}^{\beta}p_{2}^{\alpha})-(\eta_{\mu\nu}I_{\alpha\beta,\rho\sigma}+\eta_{\rho\sigma}I_{\alpha\beta,\mu\nu})p_1^\alpha p_2^\beta\\ 
&- P_{\mu\nu,\rho\sigma}(p_1\cdot p_2 -m^2)\biggr]\\
\end{split}
\end{equation}
where we have defined:
\begin{equation}
\begin{split}
   & I_{\alpha\beta,\gamma\delta}= \frac{1}{2}(\eta_{\alpha\gamma}\eta_{\beta\delta}+\eta_{\alpha\delta}\eta_{\beta\gamma}) \\
   & P_{\alpha\beta,\gamma\delta}=\frac{1}{2}(\eta_{\alpha\gamma}\eta_{\beta\delta}+\eta_{\alpha\delta}\eta_{\beta\gamma}-\frac{2}{d-2}\eta_{\alpha\beta}\eta_{\gamma\delta})
\end{split}
\end{equation}
From this action we can also extract the propagator for the scalar field, which has the usual form:
\begin{equation}
    \begin{tikzpicture}[baseline=(current bounding box.center)] \begin{feynman}
\vertex (a) {\mu};
\vertex[right =2 cm of a] (b) {\nu};
\diagram* { 
(a) -- [fermion , edge label'=\(q\)] (b),
};\end{feynman} \end{tikzpicture}=\frac{i}{q^2+i\epsilon}
\end{equation}
To get the Feynman rules for vertices involving only the graviton field we need to consider instead the Einstein-Hilbert action:
\begin{equation}
    S_{EH}=\frac{2}{\kappa^2}\int d^4x\sqrt{-g}R
\end{equation}
Since General Relativity is invariant under local coordinate transformations, it is a gauge theory and we need to quantize it.
This procedure can be done with background field method in which we expand the metric tensor as:
\begin{equation}
    g_{\mu\nu}=\Bar{g}_{\mu\nu}+\kappa h_{\mu\nu}
\end{equation}
where $\Bar{g}_{\mu\nu}$ is the classical background metric and $h_{\mu\nu}$ is the quantum field. \\
A gauge fixing condition is only imposed on the quantum field $h_{\mu\nu}$, leaving the general covariance of the background unaffected.
The calculations are greatly simplified with this method because gravitons running in the loops must be derived from an expansion involving the quantum field $h_{\mu\nu}$ whereas gravitons that are not within a loop may be derived from expanding the background field:
\begin{equation}
    \Bar{g}_{\mu\nu}= \eta_{\mu\nu}+\kappa H_{\mu\nu}
\end{equation}
where $H_{\mu\nu}$ denotes ab external graviton that is not inside a loop. \\
At the one loop level, at most two gravitons involved in a vertex are propagating within a loop, which allows us to use a gauge fixing condition linear in the quantum field $h_{\mu\nu}$ and greatly simplifies the derivation of both the triple graviton vertex and the vertex that couples one graviton to the ghost fields.\\ 
In order to fix the gauge we will use the harmonic gauge:
\begin{equation}
    \Bar{D}^{\nu}h_{\mu\nu}-\frac{1}{2}\Bar{D}_{\mu}h=0
\end{equation}
where $\Bar{D}_{\mu}$ denotes the covariant derivative on the background metric. \\
This condition leads to an additional gauge fixing piece of the action:
\begin{equation}
    S_{GF}=\int d^4x\sqrt{-\Bar{g}}\biggl(\Bar{D}^{\nu}h_{\mu\nu}-\frac{1}{2}\Bar{D}_{\mu}h\biggr)\biggl(\Bar{D}_{\rho}h^{\mu\rho}-\frac{1}{2}\Bar{D}^{\mu}h\biggr)
\end{equation}
as well as the ghost action:
\begin{equation}
    S_{Ghost}=\int d^4x\sqrt{-\Bar{g}}\Bar{\eta}^{\mu}\bigl(\Bar{D}_{\mu}\Bar{D}_{\nu}-R_{\mu\nu}\bigr)\eta^{\nu}
\end{equation}
where with $\eta^{\mu}$ and $\Bar{\eta}^{\mu}$ we denote respectively the ghost and anti-ghost particle.\\
We can now derive the Feynman rules for the effective field theory of gravity. \\
The total action is made of three pieces:
\begin{equation}
    S_{Grav}=S_{EH}+S_{GF}+S_{Ghost}
\end{equation}
By expanding it in terms of $h_{\mu\nu}$ and $H_{\mu\nu}$ we can get the desired Feynman rules.\\
The Feynman rule for the graviton propagator can be obtained by expanding at the second order the action in the quantum fields $h_{\mu\nu}$ and at zeroth order in the external gravitons $H_{\mu\nu}$ and the ghosts: 
\begin{equation}
    \begin{tikzpicture}[baseline=(current bounding box.center)] \begin{feynman}
\vertex (a) {\mu\nu};
\vertex[right =2 cm of a] (b) {\rho\sigma};
\diagram* { 
(a) -- [gluon, edge label'=\(q\)] (b),
};\end{feynman} \end{tikzpicture}= iD_{\mu\nu\rho\sigma}(q)=\frac{iP_{\mu\nu\rho\sigma}}{q^2} \qquad  
\end{equation}
We can get the ghost propagator by expanding the action to second order in the ghost fields and to zeroth order in the gravitons, obtaining:
\begin{equation}
    \begin{tikzpicture}[baseline=(current bounding box.center)] \begin{feynman}
\vertex (a) {\mu};
\vertex[right =2 cm of a] (b) {\nu};
\diagram* { 
(a) -- [charged scalar , edge label'=\(q\)] (b),
};\end{feynman} \end{tikzpicture}=iD_{\mu\nu}(q)=\frac{i\eta_{\mu\nu}}{q^2}
\end{equation}
We can then obtain the triple graviton vertex by expanding to the second order in the quantum fields $h_{\mu\nu}$ and to the first order in the background $H_{\mu\nu}$ and to zeroth order in the ghost fields and reads:
\begin{equation*}
    \begin{tikzpicture}[baseline=(current bounding box.center)] \begin{feynman}
\vertex (a) {\(\gamma\delta\)};
\vertex[below=1.5cm of a] (b) ;
\vertex[below=1.5cm of b] (c) {\(\alpha\beta\)}; 
\vertex[right=1.5cm of b] (d){\(\mu\nu\)};
\vertex[below=1cm of d] (e) ;
\vertex[above=1cm of d] (f);
\diagram* { 
(c) -- [gluon, momentum=\(k+q\)] (b)-- [gluon, momentum=\(k\)] (a),
(b) -- [gluon, momentum =\(q\)] (d) ,
};
\end{feynman} \end{tikzpicture}
\end{equation*}
\begin{equation}
\begin{split}
    \tau^{\mu\nu}_{3\alpha\beta,\gamma\delta}=\frac{-i\kappa}{2}\biggl\{&P_{\alpha\beta,\gamma\delta}\bigl[k^\mu k^\nu+(k+q)^\mu(k+q)^\nu+q^\mu q^\nu -\frac{3}{2}\eta^{\mu\nu}q^2\bigr]\\
    & +2q_\lambda q_\sigma \bigl[I^{\lambda\sigma}_{\alpha\beta}I^{\mu\nu}_{\gamma\delta}+I^{\lambda\sigma}_{\gamma\delta}I^{\mu\nu}_{\alpha\beta}-I^{\lambda\mu}_{\alpha\beta}I^{\sigma\nu}_{\gamma\delta}-I^{\sigma\nu}_{\alpha\beta}I^{\lambda\mu}_{\gamma\delta}\bigr] \\
    &+\bigl[q_{\lambda}q^\mu(\eta_{\alpha\beta}I^{\lambda\nu}_{\gamma\delta}+\eta_{\gamma\delta}I^{\lambda\nu}_{\alpha\beta})+q_\lambda q^\nu(\eta_{\alpha\beta}I^{\lambda\mu}_{\gamma\delta}+\eta_{\gamma\delta}I^{\lambda\mu}_{\alpha\beta})\\
    &-q^2(\eta_{\alpha\beta}I^{\mu\nu}_{\gamma\delta}+\eta_{\gamma\delta}I^{\mu\nu}_{\alpha\beta})-\eta^{\mu\nu}q^\lambda q^\sigma (\eta_{\alpha\beta}I_{\gamma\delta,\lambda\sigma}+\eta_{\gamma\delta}I_{\alpha\beta,\lambda\sigma})\bigr] \\
    &+\bigl[2q^\lambda(I^{\sigma\nu}_{\gamma\delta}I_{\alpha\beta\lambda\sigma}k^\mu+I^{\sigma\mu}_{\gamma\delta}I_{\alpha\beta\lambda\sigma}k^\nu-I^{\sigma\nu}_{\alpha\beta}I_{\gamma\delta,\lambda\sigma}(k+q)^\mu-I^{\sigma\mu}_{\alpha\beta}I_{\gamma\delta,\lambda\sigma}(k+q)^\nu) \\
    & +q^2(I^{\sigma\mu}_{\alpha\beta}I_{\gamma\delta,\sigma}^\nu I^{\sigma\mu}_{\gamma\delta})+\eta^{\mu\nu}q^\lambda q_\sigma(I_{\alpha\beta,\lambda\rho}I^{\rho\sigma}_{\gamma\delta}+I_{\gamma\delta,\lambda\rho}I^{\rho\sigma}_{\alpha\beta})\bigr]\\ 
    & \bigl[(k^2+(k+q)^2)\bigl(I^{\sigma\mu}_{\alpha\beta}I_{\gamma\delta,\sigma}^{\nu}+I^{\sigma\nu}_{\alpha\beta}I_{\gamma\delta,\sigma}^\mu-\frac{1}{2}\eta^{\mu\nu}P_{\alpha\beta,\gamma\delta}\bigr)-((k+q)^2\eta_{\alpha\beta}I^{\mu\nu}_{\gamma\delta}+k^2\eta_{\gamma\delta}I^{\mu\nu}_{\alpha\beta})\bigr]\biggr\}
\end{split}
\end{equation}
where the graviton with Lorentz indices $\mu\nu$ represents a background graviton and therefore it cannot be used inside a loop. \\
The Feynman rule describing the interaction between one graviton field and two ghost fields can be derived by expanding to second order in the ghost fields and to first order in $H_{\mu\nu}$:
\begin{equation}
\begin{split}
\begin{tikzpicture}[baseline=(current bounding box.center)] \begin{feynman}
\vertex (a) ;
\vertex[below=1.5cm of a] (b);
\vertex[below=1.5cm of b] (c); 
\vertex[right=1.5cm of b] (d){\(\mu\nu\)};
\vertex[below=1cm of d] (e) ;
\vertex[above=1cm of d] (f);
\diagram* { 
(c) -- [charged scalar, edge label'=\(k+q\)] (b)-- [charged scalar, edge label'=\(k\)] (a),
(b) -- [gluon, momentum =\(q\)] (d) ,
};
\end{feynman} \end{tikzpicture}= 
\tau^{\mu\nu}_{G\alpha,\beta}(k,q)=\frac{ik}{2}\biggl[& (k^2+(k+q)^2+q^2)I_{\alpha\beta}^{\mu\nu}+2\eta_{\alpha\beta}k^\lambda(k+q)^\sigma P_{\lambda\sigma}^{\mu\nu}+2q_\alpha k^\lambda I_{\beta\lambda}^{\mu\nu}\\ 
& -2q_\beta(k+q)^\lambda I_{\alpha\lambda}^{\mu\nu}+q_\alpha q_\beta \eta^{\mu\nu}\biggr]
\end{split}
\end{equation}
where the graviton with Lorentz indices $\mu\nu$ is again a background graviton and cannot be used inside a loop. \\
